# Supplementary material for: On the Benefits of Memory for Modeling Time-Dependent PDEs
Source: arXiv:2409.02313 source file (2025-04-24)
Supplement: Supplementary file 2 [file architecture.tex]

\section{Architecture Details}
\label{appendix:architecture}
\textbf{Encoder and Decoder:} For the FFNO and s4FFNO models described in section \ref{sec:architectural_details}, we use a simple grid positional encoding $E$. In 1D, if the grid has $f$ equispaced points in $[0,L]$, then $E \in \mathbb{R}^f$ and the positional encoding is defined as $E_i= \frac{i}{L}$ for $0\leq i \leq f-1$. In 2D, if we have a $f\times f$ points 2D equispaced grid in $[0,L_x]\times[0,L_y]$, the positional encoding is defined as $E_{ij} = (\frac{i}{L_x}, \frac{j}{L_y})$. In the input lifting operator $\mathcal{R}_\text{in}$, the input and the grid are stacked and a Linear layer from $\mathbb{R}^2 \rightarrow \mathbb{R}^{h_0}$ is applied element-wise. Forthe decoder $\mathcal{R}_{\text{out}}$, we use another Linear layer. 

\textbf{FFNO hyperparameters:} In our experiments, The FFNO model consists of 4 FFNO layers ($L=3$). For experiments in 1D, the hidden dimensions are all 128 ($h_j=128$ for $j=0,1,2,3$) and the expanded hidden dimension of FFNO's MLP $h'$ is $4 \cdot 128$. For experiments in 2D, the hidden dimensions are all 64 and the expanded hidden dimension is $4 \cdot 64$.  

\textbf{S4 Kernel:} The S4 repository has two available kernels, the diagonal S4 (S4D) and the Normal Plus Low Rank S4 (S4NPLR). In our experiments, we didn't find a significant difference between the two, and chose S4D for simplicity.

\textbf{TFFNO positional encoding:} In section \ref{transformer} we introduced TFFNO as a MemNO with a Transformer in the memory layer. The Transformer has causal masking and a sinusoidal positional encoding \citep{vaswani2017attention}. This positional encoding in a Transformer model is defined for each position \( pos \) in the sequence up to a maximum length \( \text{max\_len} \), and each dimension \( i \) of the encoding vector \( \text{dim\_model} \). The encoding is computed as follows:
\begin{align*}
    PE(pos, 2i) &= \sin\left(\frac{pos}{10000^{\frac{2i}{\text{dim\_model}}}}\right) \\
    PE(pos, 2i + 1) &= \cos\left(\frac{pos}{10000^{\frac{2i}{\text{dim\_model}}}}\right)
\end{align*}
