# Supplementary material for: On the Benefits of Memory for Modeling Time-Dependent PDEs
Source: arXiv:2409.02313 source file (2025-04-24)
Supplement: Supplementary file 3 [file efficient_implementation.tex]

\section{Efficient Implementation of MemNO}
\label{appendix:efficient_implementation}
